# Supplementary material for: Superior mechanical properties by exploiting size-effects and multiscale interactions in hierarchically architected foams
Source: arXiv:2207.03023 source file (2022-07-07)
Supplement: Supplementary file 1 [file Supplementary_Information_Superior.pdf]

## Supplementary Information:

### Superior mechanical properties by exploiting size-effects and multiscale interactions in hierarchically architected foams

Komal Chawla<sup>†,1</sup>, Abhishek Gupta<sup>†,2</sup>, Abhijeet S. Bhardwaj<sup>3</sup> and Ramathasan Thevamaran<sup>\*,1,2</sup>

<sup>1</sup>Department of Engineering Physics, University of Wisconsin-Madison, Madison, WI, 53706, USA.

<sup>2</sup>Department of Mechanical Engineering, University of Wisconsin-Madison, Madison, WI, 53706, USA.

<sup>3</sup>Department of Industrial and Systems Engineering, University of Wisconsin-Madison, Madison, WI, 53706, USA.

\*Corresponding author email: [thevamaran@wisc.edu](mailto:thevamaran@wisc.edu)

<sup>†</sup>These authors contributed equally to this work

#### Stress-strain curves as functions of $D_{in}$ , $t$ , and $g$

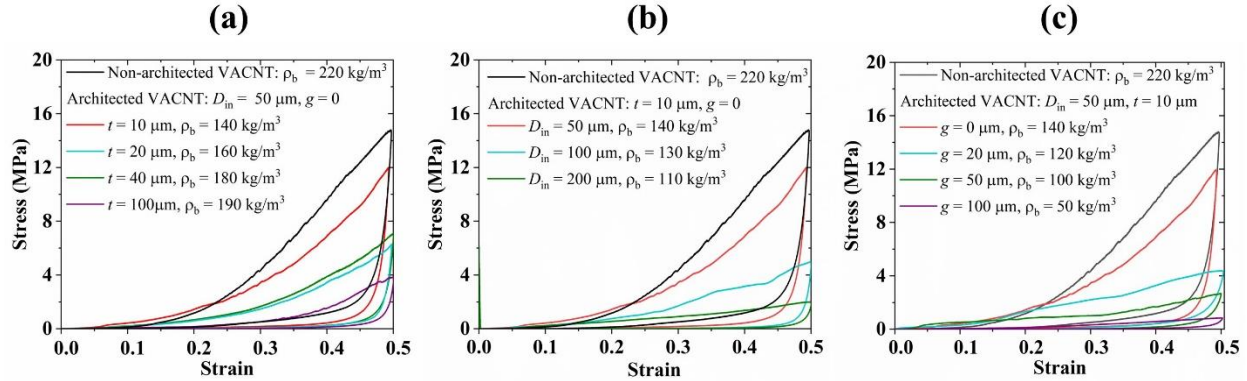

**Figure S1** (a) Stress-strain curves as a function of  $t$  for  $D_{in} = 50 \text{ } \mu\text{m}$  and  $g = 0$  compared to non-architected VACNT sample. (b) Stress-strain curves as a function of  $D_{in}$  for  $t = 10 \text{ } \mu\text{m}$  and  $g = 0$ . (c) Stress-strain curves as a function of  $g$  for  $D_{in} = 50 \text{ } \mu\text{m}$  and  $t = 10 \text{ } \mu\text{m}$ .

## Effect of intrinsic density and lateral interactions on SEA

Damping capacity  $\delta$  is the ratio of energy dissipated  $W_{dis}$  (area enclosed within the loading-unloading curve) to the total work done on the material  $W_L$  (area under the loading curve).

$$\delta = \frac{W_{dis}}{W_L} \quad (1)$$

We found the damping capacity  $\delta \approx 0.83 \pm 0.04$  for all architected VACNT foam samples independent of thickness, gap, and internal-diameter of the mesoscale cylinders. In Eq. (1),  $W_{dis}$  and  $W_L$  are in  $\text{kJ}/\text{m}^3$ , whereas  $\delta$  is a dimensionless quantity. If the bulk density of architected VACNT foam sample is  $\rho_b$ , then the specific energy absorption is defined as,

$$SEA = \frac{W_{dis}}{\rho_b} = \delta \frac{W_L}{\rho_b}$$

$$SEA = \delta \frac{1}{\rho_b} \int_0^{\epsilon_{max}} \sigma_L d\epsilon$$

where,  $\sigma_L$  is the stress response of architected VACNT foam during loading,  $\epsilon$  is the bulk strain, and  $\epsilon_{max}$  is the maximum compressive strain (0.5 in our experiments)

$$SEA = \delta \frac{1}{\rho_b} \int_0^{\epsilon_{max}} \frac{F_L}{A} d\epsilon \quad (2)$$

where,  $F_L$  is the force response of architected VACNT foam and  $A$  is the total cross-section area ( $25 \text{ mm}^2$ ). Assuming  $F_c$  is the force response from compression of an isolated cylinder and  $F_i$  is the contribution from lateral interactions with neighboring cylinders (due to cylinder's outer surface), then the total force ( $F_L$ ) is written as

$$F_L = nF_c + nF_i$$

where,  $n$  is the total number of cylinders in the sample. Substituting this in Eq. (2) yields,

$$SEA = \delta \frac{1}{\rho_b} \int_0^{\epsilon_{max}} \frac{nF_c + nF_i}{A} d\epsilon$$

$$SEA = \delta \frac{1}{\rho_b} \int_0^{\epsilon_{max}} \frac{nC_A}{A} (\sigma_c + \sigma_i) d\epsilon$$

where,  $C_A$  is the cross-section area of an individual cylinder,  $\sigma_c$  and  $\sigma_i$  are the equivalent stresses for  $F_c$  and  $F_i$ , respectively, and  $\frac{nC_A}{A} = V_f$  is the fill factor. Substituting  $V_f$  yields,

$$SEA = \delta \frac{V_f}{\rho_b} \int_0^{\epsilon_{max}} (\sigma_c + \sigma_i) d\epsilon$$

$$SEA = \delta \frac{1}{\rho_i} \int_0^{\epsilon_{max}} (\sigma_c + \sigma_i) d\epsilon$$

where,  $\rho_i = \frac{\rho_b}{V_f}$  is the intrinsic density of CNT cylinders (i.e., density of VACNT forest within the cylinders' wall region), which we found to be a function of thickness but independent of gap and internal diameter.

$$SEA = \delta \frac{1}{\rho_i} \left[ \int_0^{\epsilon_{max}} \sigma_c d\epsilon \right] + \delta \frac{1}{\rho_i} \left[ \int_0^{\epsilon_{max}} \sigma_i d\epsilon \right] \quad (3)$$

Since VACNT foams exhibit a nonlinear stress response in compression, we assume  $\sigma_c = f_1(\rho_i)f_2(\epsilon)$ . Where  $f_1(\rho_i)$  accounts for dependency of elastic modulus on intrinsic density and  $f_2(\epsilon)$  accounts for nonlinearity. We hypothesize that the stress ( $\sigma_i$ ) due to lateral interactions between outer walls of neighboring cylinders must be a function of normalized outer curved surface area  $\left(\frac{A_c}{A}\right)$ . So we assume  $\sigma_i = g_1\left(\frac{A_c}{A}\right)g_2(\epsilon)$ . Where  $g_1\left(\frac{A_c}{A}\right)$  accounts for lateral interactions and  $g_2(\epsilon)$  accounts for nonlinearities. Substituting these in Eq. (3) yields,

$$SEA = \delta f_1(\rho_i) \frac{1}{\rho_i} \int_0^{\epsilon_{max}} f_2(\epsilon) d\epsilon + \delta g_1\left(\frac{A_c}{A}\right) \frac{1}{\rho_i} \int_0^{\epsilon_{max}} g_2(\epsilon) d\epsilon$$

Integrals  $\int_0^{\epsilon_{max}} f_2(\epsilon) d\epsilon$  and  $\int_0^{\epsilon_{max}} g_2(\epsilon) d\epsilon$  are independent of design variables ( $t, g, D_{in}$ ), so assuming them to be constants, i.e.,  $\int_0^{\epsilon_{max}} f_2(\epsilon) d\epsilon = C_1$  and  $\int_0^{\epsilon_{max}} g_2(\epsilon) d\epsilon = C_2$

$$SEA = \delta f_1(\rho_i) \frac{C_1}{\rho_i} + \delta g_1\left(\frac{A_c}{A}\right) \frac{C_2}{\rho_i}$$

$$IEA = \rho_i \times SEA = \delta \left[ C_1 f_1(\rho_i) + C_2 g_1\left(\frac{A_c}{A}\right) \right] \quad (4)$$

where,  $IEA$  is the intrinsic energy absorption. On fitting the experimental data for  $D_{in} = 50 \mu m$ , we found  $C_1 \approx 2$ ,  $C_2 \approx 30.29$ ,  $f_1(\rho_i) = \rho_i$ , and  $g_2\left(\frac{A_c}{A}\right) = \left(\frac{A_c}{A}\right)^{1.125}$

Normalized curved surface area of cylinders can be calculated as follows

$$\frac{A_c}{A} = \pi(D_{in} + 2t)h \left[ \frac{1}{\sqrt{3}(g + D_{in} + 2t)^2} - \frac{1}{3\sqrt{A}} \frac{1}{(D_{in} + 2t + g)} \right]$$

The subtracting term is the normalized outer curved surface area of cylinders at the perimeter of the sample, and  $h$  is the height of the VACNT foam sample.

### Scaled modulus and scaled peak stress

Similar to  $SEA$ , the trend reversal in  $t: g$  parameter interaction plots of  $E^*$  and  $\sigma_p^*$  disappears after multiplying them by the intrinsic density ( $\rho_i$ ), underscoring the competing effects between size-effect and the effect of interaction among adjacent cylinders. Scaled modulus ( $= E^* \times \rho_i$ ) and scaled peak stress ( $= \sigma_p^* \times \rho_i$ ) are plotted in Figure S2 below

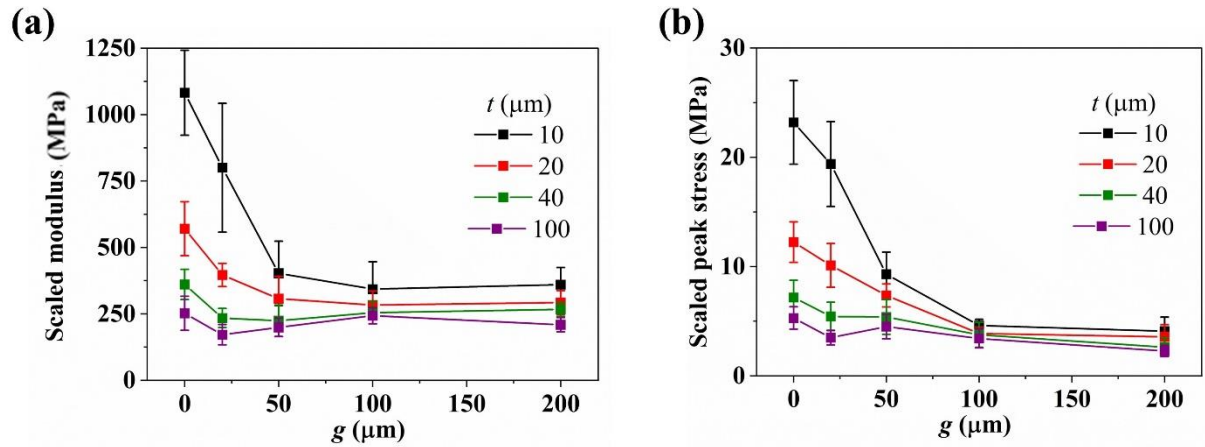

**Figure S2** (a) Scaled modulus and (b) scaled peak stress as functions of  $t$  and  $g$ .

## Relationship between $SEA$ , $\sigma_p^*$ , and $E^*$

Let the area under the unloading curve (work done by the material) be  $W_{UL}$ , then

$$W_L = W_{dis} + W_{UL}$$

$$\frac{W_L}{W_{dis}} = 1 + \frac{W_{UL}}{W_{dis}}$$

$$\frac{1}{\delta} = 1 + \frac{W_{UL}}{W_{dis}}$$

$$\frac{SEA \times \rho_b}{W_{UL}} = \frac{\delta}{1 - \delta} \quad (W_{dis} = SEA \times \rho_b)$$

$W_{UL}$  can be calculated by adding the area under the unloading curve in three different regimes of strain [1] as shown in Figure S3.

$$W_{UL} = \int_0^{\epsilon_p} 0 \times d\epsilon + \int_{\epsilon_p}^{\epsilon_m} \sigma_1 d\epsilon + \int_{\epsilon_m}^{\epsilon_{max}} \sigma_2 d\epsilon$$

Where  $\epsilon_p$  is the permanent strain,  $\epsilon_m$  is the strain at the intersection of two approximated linear regimes ( $0.48 < \epsilon_m < 0.49$ ) shown in Figure S3, and  $\epsilon_{max}$  is the maximum compressive strain ( $\epsilon_{max} = 0.5$ )

$$\sigma_1 = (\epsilon - \epsilon_p) \frac{(\sigma_p + E_{UL}(\epsilon_m - \epsilon_{max}))}{(\epsilon_m - \epsilon_p)}, \quad \sigma_2 = \sigma_p + E_{UL}(\epsilon - \epsilon_{max})$$

where,  $\sigma_1$  is the linear fit for stress as a function of strain in the first linear regime and  $\sigma_2$  is the linear fit for stress as a function of strain in the second linear regime (Figure S3).  $E_{UL}$  is the unloading modulus and  $\sigma_p$  is the peak stress.

$$W_{UL} = \sigma_p \left[ \frac{2\epsilon_{max} - \epsilon_m - \epsilon_p}{2} \right] - E_{UL} \left[ \frac{(\epsilon_{max} - \epsilon_m)(\epsilon_{max} - \epsilon_p)}{2} \right]$$

$$SEA = \frac{\delta}{1 - \delta} \times \left[ \sigma_p^* \left[ \frac{2\epsilon_{max} - \epsilon_m - \epsilon_p}{2} \right] - E^* \left[ \frac{(\epsilon_{max} - \epsilon_m)(\epsilon_{max} - \epsilon_p)}{2} \right] \right] \quad (5)$$

where,  $\sigma_p^* = \frac{\sigma_p}{\rho_b}$  is the specific peak stress and  $E^* = \frac{E_{UL}}{\rho_b}$  is the specific modulus

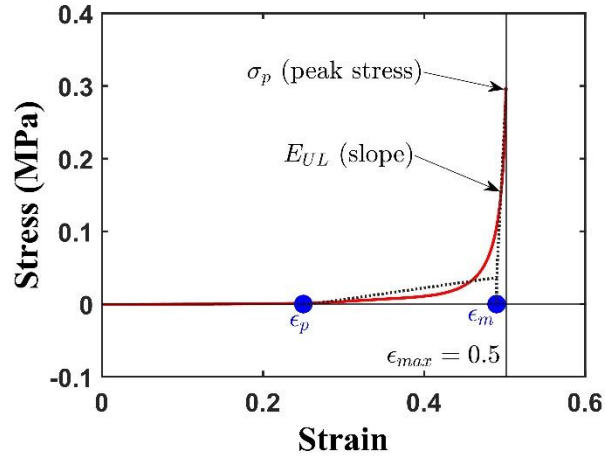

**Figure S3** Typical unloading curve for VACNT foam sample with three different strain regimes indicated ( $\epsilon_{max}$  to  $\epsilon_m$ ,  $\epsilon_m$  to  $\epsilon_p$ ,  $\epsilon_p$  to 0). Nonlinearity is approximated by dividing the curve into two intersecting linear fits.

## Effect of thickness on deformation mechanism

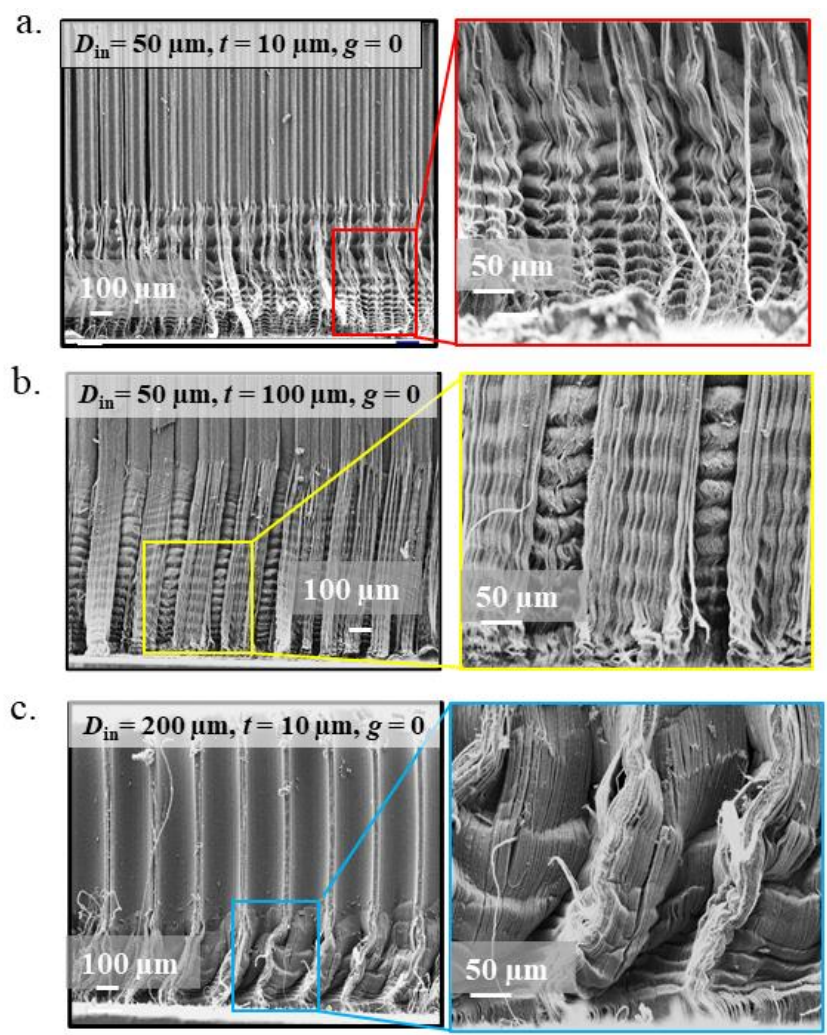

**Figure S4** SEM images of compressed architected samples post recovery with (a)  $D_{in} = 50 \mu\text{m}$ ,  $t = 10 \mu\text{m}$  (b)  $D_{in} = 50 \mu\text{m}$ ,  $t = 100 \mu\text{m}$  and (c)  $D_{in} = 200 \mu\text{m}$ ,  $t = 10 \mu\text{m}$ . Portions of the samples exhibit permanent deformation in the form of partially recovered collective buckles of CNTs. Samples with 50  $\mu\text{m}$  inner diameter and 10  $\mu\text{m}$  thickness shows large number of buckles of much smaller wavelengths compared to the samples with 200  $\mu\text{m}$  inner diameter and 100  $\mu\text{m}$  thickness.

## Effect of $D/t$ ratio on SEA

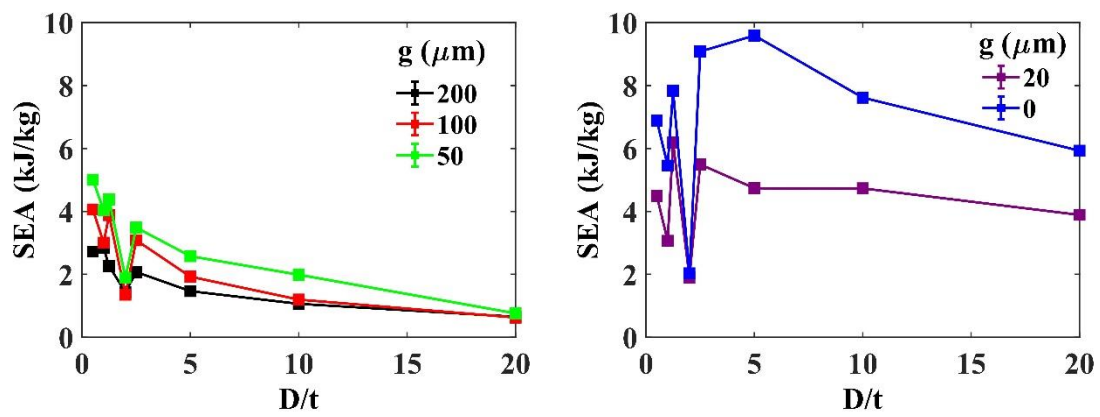

**Figure S5** SEA as a function of  $D/t$  ratio for different gaps ( $g$ )

## Steps to develop statistical model for SEA

We study the dependence of response variables on design variables using Analysis of Variance (ANOVA) model. The choice of using ANOVA is appropriate as we discretize the continuous design variables at fixed levels in our experimental setup while synthesizing VACNT samples. Here, we provide a step-by-step guide of selecting the best ANOVA model for response variable SEA. As we have three repetitions for each combination of design variables, we begin the analysis by generating full factor ANOVA model where all interactions terms are allowed to exist in the model. We do not consider any transformation of the response variable in the initial full model. Table S1 shows that all the factors and interaction terms for the full factor ANOVA model without transformation are statistically significant. However, statistical significance of independent variables is not sufficient to judge the fit of the model and thus we diagnose the full model by generating diagnostic plots for it as shown in Figure S6. For a good ANOVA model, it is important that all the assumptions of ANOVA are met appropriately. The diagnostic plots help to visualize the discrepancy faced in meeting the assumption of ANOVA model. As can be seen in Figure S6(a) the assumption of ‘homoscedasticity of residuals’ is violated by the full ANOVA model. Also, as seen in Figure S6(b) the residuals are not ‘normally distributed’ and have some linear dependency among them as seen in Figure S6(c), thus violating the assumption of ‘independence of residuals’. Further, Figure S6(d) also present a suspicious outlier in the dataset, which does not make much sense in an experimental setup as ours and instead apply poor model fitting by the full model without appropriate transformations.

|           | SumSq  | Df  | Fvalue  | Pr(>F)   | Significance |
|-----------|--------|-----|---------|----------|--------------|
| Intercept | 2577.0 | 1   | 3648.00 | <2.2e-16 | ***          |
| Din       | 338.0  | 2   | 239.26  | <2.2e-16 | ***          |
| t         | 31.2   | 3   | 14.74   | 3.13E-08 | ***          |
| Gap       | 788.1  | 4   | 278.92  | <2.2e-16 | ***          |
| Din:t     | 8.2    | 6   | 1.94    | 0.08002  | .            |
| Din:Gap   | 86.5   | 8   | 15.31   | 2.50E-15 | ***          |
| t:Gap     | 221.9  | 12  | 26.17   | <2.2e-16 | ***          |
| Din:t:Gap | 33.6   | 24  | 1.98    | 0.0086   | **           |
| Residuals | 84.8   | 120 |         |          |              |

**Table S1** ANOVA table for full factor model

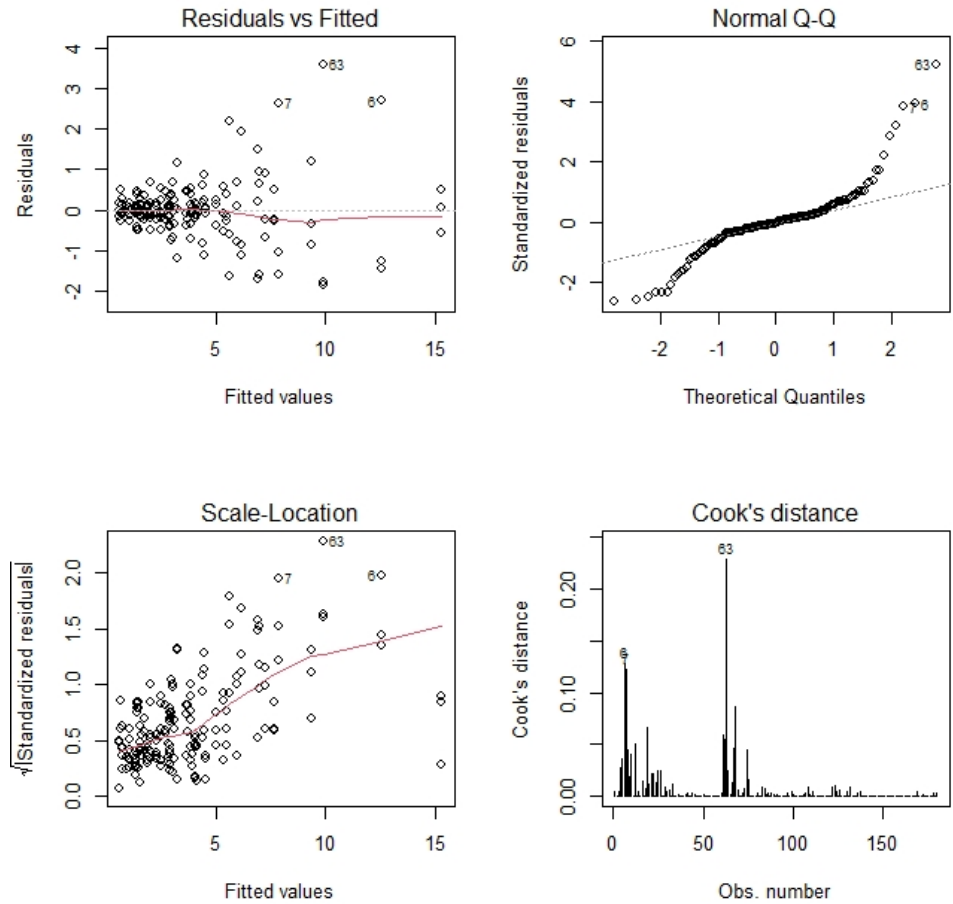

**Figure S6** Model diagnostics: (a) residual versus fitted, (b) normal Q-Q, (c) scale-location and (d) Cook's distance plots.

As ANOVA assumptions are not met appropriately in the initial model, we improve the same by considering different transformations for the response variables and also eliminate the lower-level interaction terms to honor model parsimony. We consider log transformation and Box-Cox transformation for the response variable. Our major goal is to improve model fit by selecting model that meet ANOVA assumptions at best. To quantify how well do each model meet ANOVA assumption we make use of the following statistical tests.

1. **Durbin-Watson Test**: This test helps to check if there is some trend or autocorrelation in the residual. A good fit ANOVA model do not have autocorrelation of residuals. We perform the test in R programming language where the null hypothesis is that residuals do

not have correlation. A p-value  $>0.05$  implies insufficient evidence to reject null hypothesis and thus imply absence of autocorrelation.

2. Breusch-Pagan (BP) Test: We use this test to check homoscedasticity of residuals. The null hypothesis of the BP-Test assumes homoscedasticity of residuals and if the p-value is larger than an appropriate threshold, ( $>0.05$ ) then we fail to reject the null hypothesis and conclude that residuals adhere to the assumption of homoscedasticity.
3. Shapiro-Wilk Test: We use this test to check if the residuals are normally distributed or not. The null hypothesis for the test is that data is normally distributed and having a p-value above a threshold ( $>0.05$ ) would imply normality of residuals.

We evaluate p-values for all the tests mentioned above for different models. The reduced models are achieved by only selecting statistically significant terms from the ANOVA of the full model. Finally, if higher order interactions are significant, we only select them instead of lower order terms to respect model parsimony and ease model interpretation. We demonstrate the test results for different models of SEA in Table S2. As can be seen from Table S2 reduced model with Box-Cox transformation and Parsimonious Model with only higher order interaction terms give positive results for all the three tests validating ANOVA assumption. We finally plot the diagnostic plot of the best fit model (Parsimonious model with Box-Cox transformation) in Figure S7. As can be seen the diagnostic plots provide much improved results as compared to Figure S6 thus affirming the best fit model.

| <i><b>Model Type</b></i>                  | <i><b>Transformation</b></i> | <i><b>Durbin Watson Test</b></i> | <i><b>Breusch Pagan Test</b></i> | <i><b>Shapiro wilks test</b></i> | <i><b>Independent Variables</b></i> |
|-------------------------------------------|------------------------------|----------------------------------|----------------------------------|----------------------------------|-------------------------------------|
| Full-Model                                | --                           | 0.00200                          | 0.00000                          | 0.00000                          |                                     |
| Full-Model                                | Logarithm                    | 0.16800                          | 0.00334                          | 0.00038                          |                                     |
| Reduced-Model                             | Logarithm                    | 0.08200                          | 0.02703                          | 0.03170                          | Din+Gap+t:Gap+<br>Din:t+Din:Gap     |
| Full-Model                                | Box-Cox                      | 0.12800                          | 0.93623                          | 0.00736                          |                                     |
| Reduced-Model                             | Box-Cox                      | <b>0.09600</b>                   | <b>0.57578</b>                   | <b>0.67743</b>                   | Din+Gap+Din:Ga<br>p+t:Gap           |
| Model with<br>higher order<br>interaction | Box-Cox                      | <b>0.08800</b>                   | <b>0.57578</b>                   | <b>0.67743</b>                   | Din:Gap+t:Gap                       |

**Table S2** Model selection using tests for validating ANOVA assumptions.

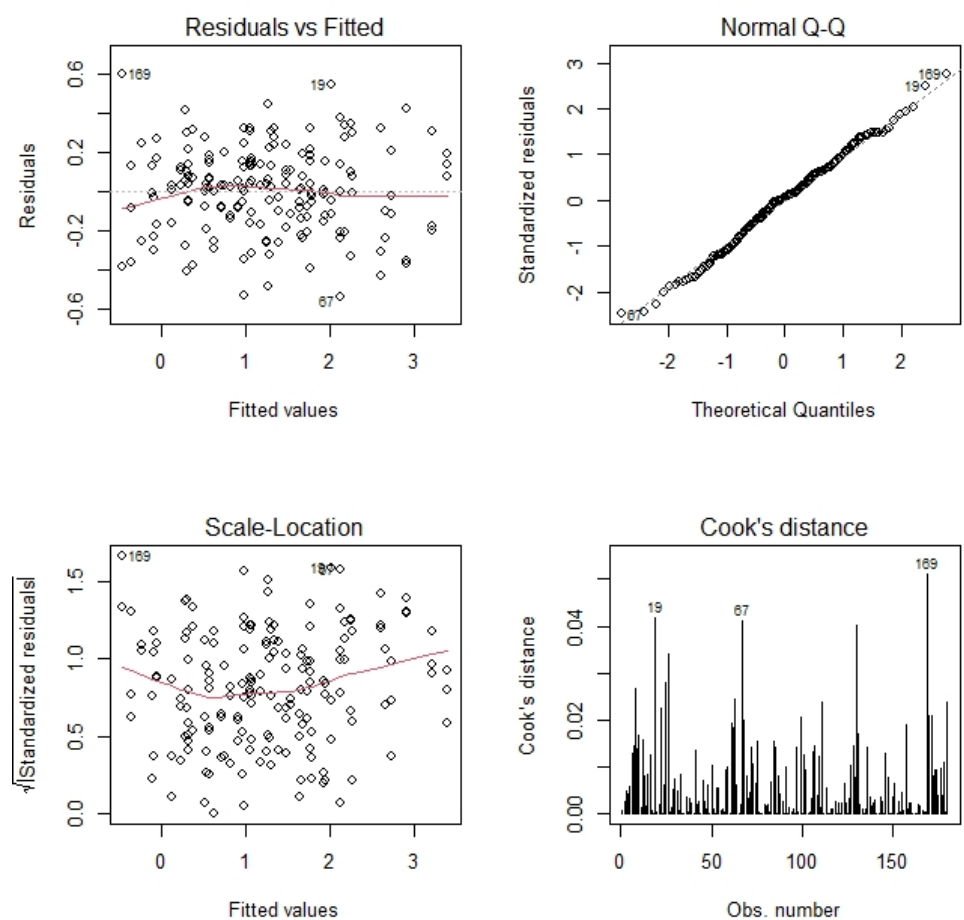

**Figure S7** Model diagnostics: (a) residual versus fitted, (b) normal Q-Q, (c) scale-location and (d) Cook's distance plots for parsimonious model with Box-Cox transformation.

## Bibliography

- [1] J. Suhr *et al.*, "Fatigue resistance of aligned carbon nanotube arrays under cyclic compression," *Nature Nanotechnology*, vol. 2, no. 7, 2007, doi: 10.1038/nnano.2007.186.
